# Supplementary material for: 3D-Consistent Image Inpainting with Diffusion Models
Source: arXiv:2412.05881 source file (2024-12-08)
Supplement: Supplementary file 1 [file supplementary.tex]

\clearpage
\setcounter{page}{1}
\maketitlesupplementary

%===============================================================
\PAR{More qualitative results}
We here complement visual inpainting examples for the evaluation datasets.
In Figures~\ref{fig:supp1}-\ref{fig:supp2} we present qualitative examples of inpainting for four datasets. For the random masks, our samples produce 3D consistent inpaintings and the overall harmonized boundaries between the masked ans known regions.

%------------------------------------------
\begin{figure}[t!] \centering   
    \begin{tabular}{cccc}
    Origin & \quad \quad Mask & \quad In-context  & \ Inpainting \\
    \end{tabular}
\includegraphics[width=0.99\columnwidth]{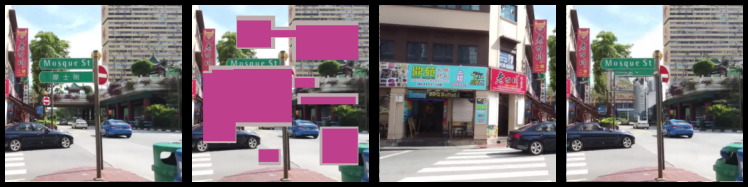}
\includegraphics[width=0.99\columnwidth]{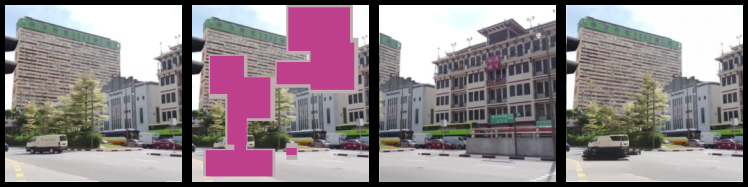}
\includegraphics[width=0.99\columnwidth]{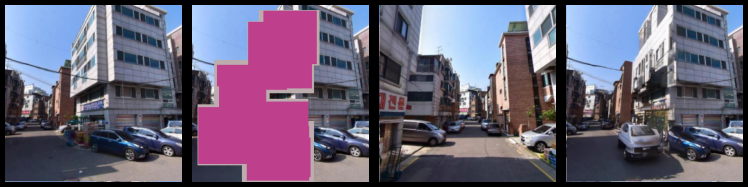}
\includegraphics[width=0.99\columnwidth]{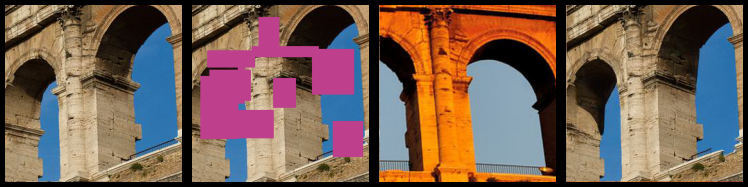}
\includegraphics[width=0.99\columnwidth]{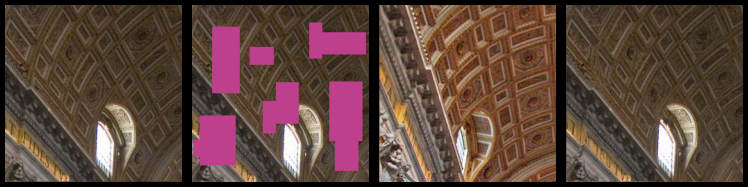}
\includegraphics[width=0.99\columnwidth]{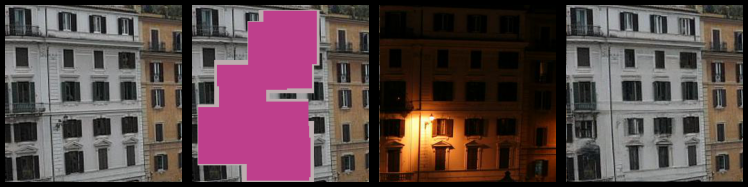}
\caption{\label{fig:supp1}StreetView and MegaDepth datasets: inpainting with random masks.}    
\end{figure}

\begin{figure}[t!] \centering    
    \begin{tabular}{cccc}
    Origin & \quad \quad Mask & \quad In-context  & \ Inpainting \\
    \end{tabular}
    \includegraphics[width=0.99\columnwidth]{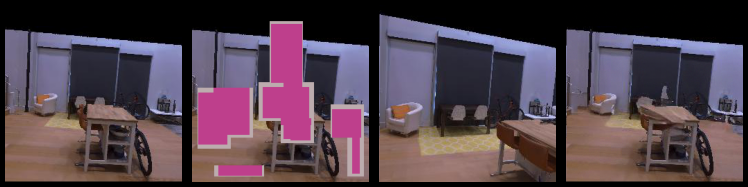}
    \includegraphics[width=0.99\columnwidth]{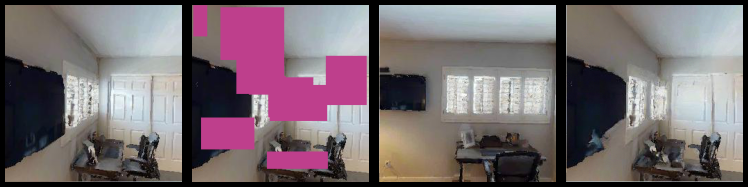}
    \includegraphics[width=0.99\columnwidth]{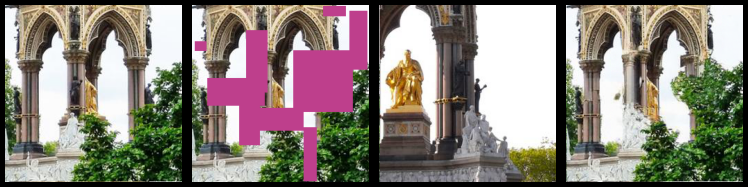}
    \includegraphics[width=0.99\columnwidth]{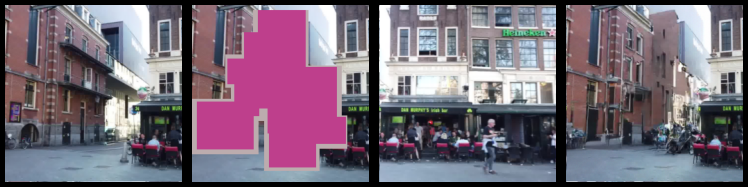}
    \includegraphics[width=0.99\columnwidth]{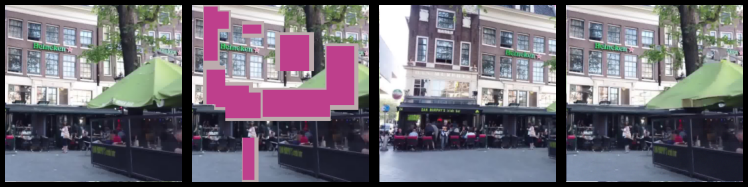}
    \includegraphics[width=0.99\columnwidth]{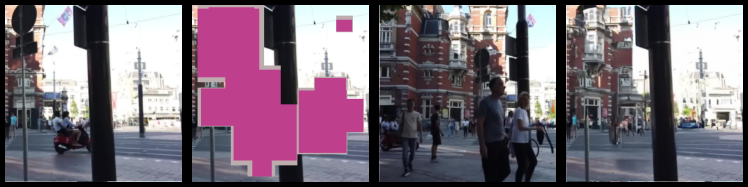}
    \caption{\label{fig:supp2} HM3D and WalkingTour datasets: inpainting with random masks.}    
\end{figure}
%----------------------------------------------

\input{tables/teaser_vs_SD}
%--------------------------------------------------------
\PAR{Inpainting with \name \ vs SD-XL}
As mentioned in the main paper, using Stable Diffusion models in complex real-world scenes can produce irrealistic and off-context inpaintings. Figure~\ref{fig:teaser_SD} shows some of such examples and compare them to \name \ inpainting, trained with an additional viewpoint of the scene that 
makes inpainting more realistic and 3D-consistent. 
The figure shows the original image, image with masked occlusions, in-context image, \name \ inpainting and finally SD-XL inpainting for the same mask.    

%--------------------------------------------------------
\PAR{Compute time}
Stable Diffusion models are trained using considerable computing resources and very large datasets.
Compute time to train a Stable Diffusion model from scratch takes 79,000 NVIDIA A100-hours in 13 days, for a total training cost of $\$160k$. For comparison, training a \name \ model takes 15 days on just 1 NVIDIA A100 GPU. .
